# Supplementary material for: Neutrino Fast Flavor Conversions in Neutron-star Post-Merger Accretion Disks
Source: arXiv:2103.02616 ancillary file (2021-05-27)
Supplement: Supplementary file 1 [file supplementary_material.pdf]

# Supplementary Material

Xinyu Li (李昕宇) [1,2*] and Daniel M. Siegel[1,3]
[1] *Perimeter Institute for Theoretical Physics, Waterloo, Ontario, Canada, N2L 2Y5*
[2] *Canadian Institute for Theoretical Astrophysics, Toronto, Ontario, Canada, M5R 2M8*
[3] *Department of Physics, University of Guelph, Guelph, Ontario, Canada, N1G 2W1*

*Neutrino Transport* — In a 3+1 decomposed spacetime with 4-metric $g_{\alpha\beta}$, timelike normal vector $n^\alpha$ and spatial metric $\gamma_{\alpha\beta}$, the stress energy tensor of neutrino radiation in a two-moment approximation [1, 2] can be written as

$$T^{\alpha\beta}_{\rm rad} = J u^\alpha u^\beta + H^\alpha u^\beta + H^\beta u^\alpha + L^{\alpha\beta} \tag{1}$$

or

$$T^{\alpha\beta}_{\rm rad} = E n^\alpha n^\beta + F^\alpha n^\beta + F^\beta n^\alpha + P^{\alpha\beta}, \tag{2}$$

where $u^\alpha$ is the fluid 4-velocity. $J$, $H^\alpha$ and $L^{\alpha\beta}$ are the zero, one and two moments of the neutrino radiation field in the fluid frame, with $H^\alpha u_\alpha = L^{\alpha\beta} u_\alpha = 0$. Furthermore, $E$, $F^\alpha$, $P^{\alpha\beta}$ are the corresponding moments in the lab frame (Eulerian observer), with $F^\alpha n_\alpha = P^{\alpha\beta} n_\alpha = 0$ and, therefore, $F^0 = P^{0\alpha} = 0$. The moments in different frames are related through

$$E = W^2 J + 2W H^\alpha v_\alpha + L^{\alpha\beta} v_\alpha v_n u, \tag{3}$$
$$F_i = W\left(J + H_i v^i\right) v_i + W H_i - \gamma^\alpha_i n^\beta L_{\alpha\beta}, \tag{4}$$

where $W = -u^\alpha n_\alpha$ is the Lorentz factor and $v_i = u_i/W$ are the covariant components of the 3-velocity, with $v^i = \gamma^{ij} v_i$.

The evolution equations for $E$ and $F_i$ in conservative form are written as

$$\partial_t(\sqrt{\gamma}E) + \partial_j\left[\sqrt{\gamma}\left(\alpha F^j - \beta^j E\right)\right] = \alpha\sqrt{\gamma}\left(P^{ij}K_{ij} - F^j \partial_j \ln\alpha - S^\alpha n_\alpha\right), \tag{5}$$
$$\partial_t(\sqrt{\gamma}F_i) + \partial_j\left[\sqrt{\gamma}\left(\alpha P^j_i - \beta^j F_i\right)\right] = \sqrt{\gamma}\left(-E\partial_i\alpha + F_k\partial_j\beta^k + \frac{\alpha}{2}P^{jk}\partial_i\gamma_{jk} + \alpha S^\alpha \gamma_{i\alpha}\right), \tag{6}$$

where $\alpha$ and $\beta^i$ are the lapse and shift, and $\gamma = \det(\gamma_{ij})$. Higher radiation moments are neglected in this M1 approach; $P^{ij}$ is determined through a closure relation $P^{ij}(E, F_i)$ that interpolates between the optically thin and thick limit,

$$P^{ij} = \frac{3\chi - 1}{2}\left(E\frac{F^i F^j}{\gamma_{ij}F^i F^j}\right) + \frac{3(1-\chi)}{2}\left[\frac{J}{3}\left(\gamma^{ij} + 4W^2 v^i v^j\right) + W(H^i v^j + H^j v^i)\right], \tag{7}$$

where

$$\chi = \frac{3 + 4\bar{F}^2}{5 + 2\sqrt{4 - 3\bar{F}^2}}, \tag{8}$$

with

$$\bar{F}^2 = \frac{h_{\alpha\beta}H^\alpha H^\beta}{J^2} \tag{9}$$

and $h_{\alpha\beta} = g_{\alpha\beta} + u_\alpha u_\beta$.

The collisional source term $S^\alpha$ is given by

$$S^\alpha = \eta u^\alpha - \kappa_a J u^\alpha - (\kappa_a + \kappa_s) H^\alpha, \tag{10}$$

where $\eta$ is the neutrino emissivity, $\kappa_a$ and $\kappa_s$ denote the opacity from absorption and scattering, respectively, provided by `NuLib` [3].

The `NuLib` data provide neutrino emissivities and absorption opacities as well as elastic and inelastic inelastic scattering opacities. Neutrino emission includes electron capture on protons and nuclei as well as positron captures onto neutrons, electron-positron pair annihilation, and nucleon-nucleon Bremsstrahlung. The absorption opacity includes absorption of $\nu_e$ by neutrons and heavy nuclei, and absorption of $\bar{\nu}_e$ by protons. Scattering opacities involve elastic neutrino scattering on neutrons, protons, heavy nuclei, and alpha particles, and inelastic electron-neutrino scattering. The details of neutrino-matter interactions can be found in Section 3 of Ref. [3] (see their Table 1 for a summary).

* xli@cita.utoronto.ca

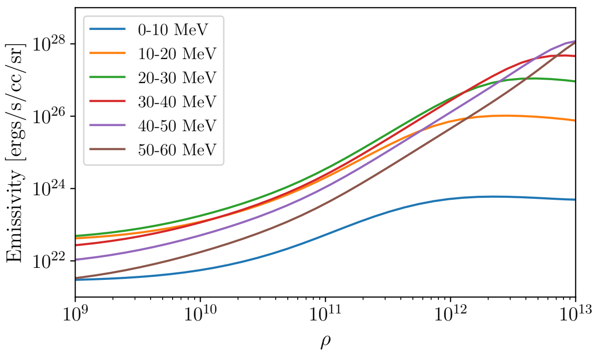


Figure 1. Neutrino emissivities for $\nu_e$ at typical accretion disk conditions ($T = 5$ MeV and $Y_e = 0.1$) for each energy bin.

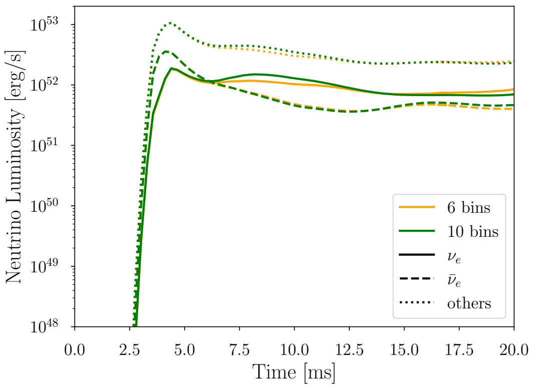


Figure 2. Neutrino luminosity of the `FC` run, using six and ten energy bins for M1 transport, showing consistent results. Luminosities are extracted at a radius of 1000 km.

In our simulations, we describe each neutrino species by six energy bins, equally spaced between 0 and 60 MeV, and evolve $E_{(\nu)}$ and $F_{(\nu)i}$ for each energy group accordingly. Fig. 1 shows the emissivities of $\nu_e$ for each energy bin at $T = 5$ MeV and $Y_e = 0.1$, which represent typical conditions of our simulated accretion disks. The emissivities peak at $20 - 30$ MeV and emission in the low energy bin below 10 MeV is reduced by typically one or more orders of magnitude. Neutrinos above 60 MeV are strongly suppressed and their absorption opacity can become very large; these are immediately reabsorbed 'on the spot' and their non-local effects in setting disk outflow properties are thus unimportant. High absorption opacity also poses a numerical challenge in that the source term becomes stiff. In this case, we replace $J$ and $H^{\alpha}$ in Equation (10) with $E$ and $F^i$. This approximation is valid for small $u^i$, but may cause significant error for large $u^i$. Such excessively large absorption opacities only occur in our highest-energy bin, the high-energy tail of the neutrino spectrum.

A convergence test using ten energy bins for the neutrino spectrum in the range $0 - 60$ MeV has been performed for the first 20 ms of evolution. This run, which is otherwise identical to our fiducial `FC` run, yields consistent results, indicating that six energy bins are appropriate for this system. As an indicator for non-local transport effects, Fig. 2 compares the total neutrino luminosities of these two runs, showing good agreement. As $\nu_e$ and $\bar{\nu}_e$ are more copiously produced, neutrino fast flavor conversions essentially reduce the luminosity for $\nu_e$ and $\bar{\nu}_e$ and increase the luminosity of the other species. Luminosities of both runs are consistent for all species. They do not depend on the radius at which they are extracted numerically, as long as the extraction surface is placed sufficiently far from the emission and absorption region.

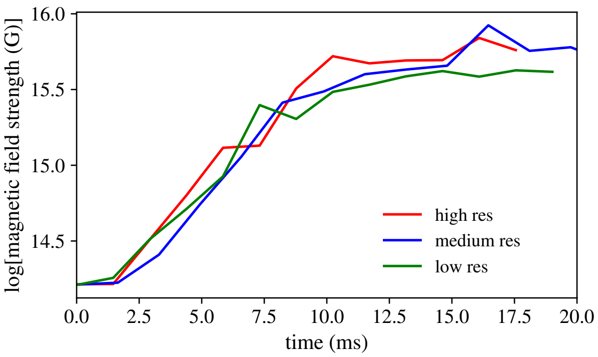


Figure 3. Initial amplification of the magnetic field (maximum in the meridional (xz) plane). The saturation level is consistent among simulations including fast conversions at low, medium, and high resolution (1.7 km, 1.3 km, and 0.85 km), indicating convergence of our fiducial simulations at medium resolution.

*Convergence Test* — The magneto-rotational instability leads to an exponential growth phase of the magnetic field from its initial seed value until saturation is reached around 15 ms (Fig. 3). The saturation level is consistent among different resolutions employed (Fig. 3), indicating convergence of our simulations at the fiducial resolution of 1.3 km.

*Accretion Rate* — After an initial relaxation phase, the disk resides in a quasi-steady turbulent accretion state. Figure 4 shows the accretion rate, measured at a radius of $\approx 20$ km, after 20 ms when the quasi-steady turbulent accretion state is established. Initially, the accretion rate starts at 1 $M_{\odot}\mathrm{s}^{-1}$ and decreases to 0.01 $M_{\odot}\mathrm{s}^{-1}$ at around 400 ms as a result of secular evolution (viscous spreading).

*Angular Distribution of the Ejecta* — Figure 5 shows the angular distribution of the cumulative unbound disk outflow across a spherical surface with radius 700 km centred on the black hole until 400 ms. Here, $\theta$ is the polar angle from the equatorial plane, where $\sin\theta = 0$ corresponds to the equatorial plane and $\sin\theta = 1$ corresponds to the pole along the $z$ axis. Only $\approx 0.2\%$ of the ejecta is launched in the range $\sin\theta > 0.9$, i.e. within 26° from

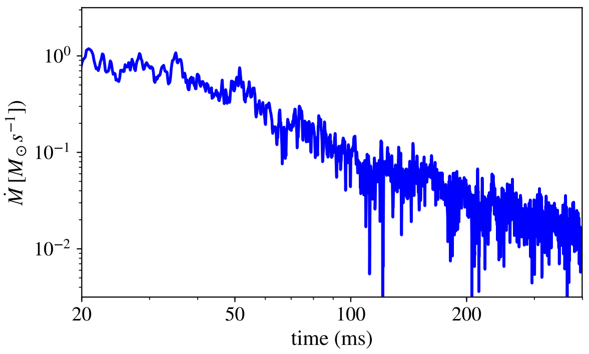


Figure 4. Accretion rate onto the black hole after 20 ms when the disk has relaxed into a quasi-stationary state, measured as the mass flow through a detector surface at a radius of $\approx$20 km.

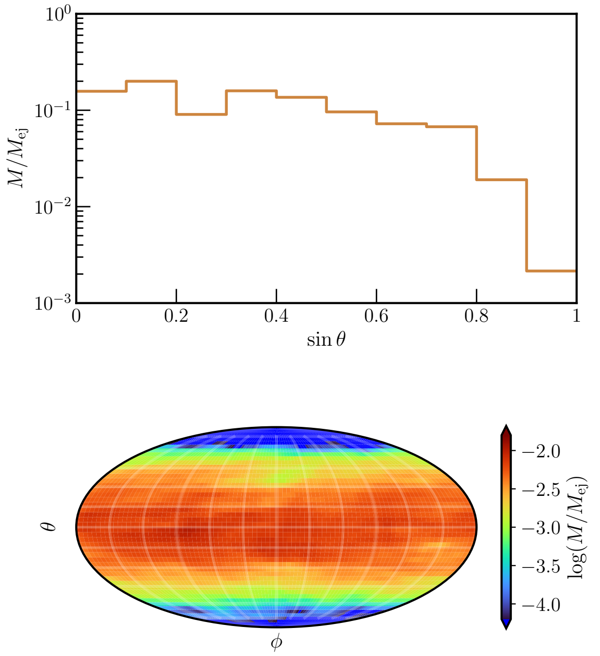


Figure 5. Top: angular distribution of the cumulative ejecta passing through a detector surface of radius 700 km until 400 ms. The angle $\theta$ denotes the polar angle from the equator. Bottom: corresponding 2D angular distribution of cumulative ejecta.

the $z$ axis, indicating that only a small fraction of the ejecta is launched from the polar region. This conclusion is independent of the distance employed for the ejecta sphere.

[1] K. S. Thorne, MNRAS **194**, 439 (1981).
[2] M. Shibata, K. Kiuchi, Y. Sekiguchi, and Y. Suwa, Progress of Theoretical Physics **125**, 1255 (2011), arXiv:1104.3937 [astro-ph.HE].
[3] E. O'Connor, ApJS **219**, 24 (2015), arXiv:1411.7058 [astro-ph.HE].
